# Supplementary material for: Does Your Reasoning Model Implicitly Know When to Stop Thinking?
Source: arXiv:2602.08354 source file (2026-05-16)
Supplement: Supplementary file 1 [file sagerebuttalappendix.tex]

\section{Additional Results and Clarifications from the Rebuttal}
\label{app:rebuttal}

In response to the reviewers' questions, we conducted additional analyses and experiments to clarify the generality of SAGE, the transition from token-wise search to step-wise exploration, the training and evaluation protocol, and the comparison with efficient-reasoning baselines. We summarize these additions below and will incorporate them into the camera-ready version.

\subsection{Generalization of the Motivation Beyond MATH-500}
\label{app:motivation_generalization}

The reviewers asked whether the motivating observation behind SAGE generalizes beyond MATH-500 and AMC23. To address this, we analyzed the rank of the end-of-thinking token under TSearch with $\Phi$ on AIME and OlympiadBench using DS-1.5B and DeepScaleR. The end-of-thinking token remains ranked first on average, supporting the claim that high-confidence reasoning paths tend to terminate earlier. We further evaluated SAGE on broader benchmarks, as shown in Table~\ref{tab:rebuttal_generalization}.

\begin{table}[t]
  \centering
  \caption{Generalization results on OlympiadBench and AIME 2024. SAGE achieves clear accuracy gains while reducing average response length compared with Degrade-SAGE.}
  \label{tab:rebuttal_generalization}
  \begin{tabular}{llrrrr}
    \toprule
    Model & Method &
    \multicolumn{2}{c}{OlympiadBench} & \multicolumn{2}{c}{AIME 2024} \\
    \cmidrule(lr){3-4} \cmidrule(lr){5-6}
    & & Pass@1 & Len. & Pass@1 & Len. \\
    \midrule
    DS-1.5B & SAGE (2,1) & 38.7 & 4833 & 30.3 & 6840 \\
    DS-1.5B & Degrade-SAGE & 33.8 & 8942 & 26.1 & 12537 \\
    DeepScaleR & SAGE (2,1) & 39.1 & 4211 & 36.4 & 7798 \\
    DeepScaleR & Degrade-SAGE & 36.1 & 6053 & 31.7 & 9444 \\
    \bottomrule
  \end{tabular}
\end{table}

\subsection{From Token-Wise Search to Step-Wise Exploration}
\label{app:stepwise_search}

Reviewers requested a clearer justification for replacing token-wise TSearch with step-wise SAGE. We clarify that a reasoning step is defined as a complete reasoning segment generated by the model, ending at a natural step boundary or the end-of-thinking token. Since the end-of-thinking token appears at the end of a reasoning step rather than at an arbitrary token position, token-wise and step-wise exploration are aligned for the termination decision.

We also examined whether token-level exploration inside a reasoning step is necessary. For each problem, we sampled complete-step prefixes and random-position prefixes, then ran TSearch from these prefixes and encoded candidates with all-MiniLM-L6-v2. Candidate branches starting from random positions inside a step were substantially more similar than those starting from complete steps, indicating that token-level search inside a step contributes little diversity.

\begin{table}[t]
  \centering
  \caption{Similarity among branches generated from different prefix types. Higher similarity for random-position prefixes suggests that token-level search inside reasoning steps is less useful than step-level branching.}
  \label{tab:rebuttal_step_similarity}
  \begin{tabular}{lc}
    \toprule
    Prefix type & Similarity \\
    \midrule
    Complete steps & 0.6883 \\
    Random positions & 0.8897 \\
    \bottomrule
  \end{tabular}
\end{table}

Finally, we compared token-wise TSearch and step-wise SAGE under aligned settings. As Table~\ref{tab:rebuttal_tsearch_sage} shows, SAGE closely matches TSearch in accuracy while avoiding expensive token-level candidate maintenance.

\begin{table}[t]
  \centering
  \caption{Token-wise TSearch and step-wise SAGE under aligned settings.}
  \label{tab:rebuttal_tsearch_sage}
  \begin{tabular}{lrrrr}
    \toprule
    Method & TR & Acc. & T-Len. & Len. \\
    \midrule
    TSearch (4,1) w/ $\Phi$ & 1.00 & 0.92 & 2213 & 2609 \\
    SAGE (4,1) & -- & 0.92 & 2234 & 2655 \\
    \bottomrule
  \end{tabular}
\end{table}

\subsection{Exploration Width, Step Budget, and RL Training Settings}
\label{app:ew_training_settings}

Reviewers asked whether the exploration width (EW) and step budget were too narrow. We found that TSearch performance converges clearly as EW increases from 1 to 6, making EW=6 a reasonable maximum in our setting. In addition, vLLM only supports up to top-16 log-probabilities per token; when EW=6, we keep top-12 log-probabilities per token, so substantially larger EW values would preserve very low-rank tokens with limited practical value. We also analyzed SAGE with step budgets from 10 to 80 and found the reported configuration to be a good cost-performance trade-off.

For RL training, we use a group size of 8, following common practice in the LLM-RL literature. Increasing EW sharply raises latency after EW exceeds 2, while performance gains become marginal. Under our setting, the difference between using two or one SAGE trajectories is negligible, and using EW=2 gives the best cost-performance trade-off. We apply the same token budget to all baselines to ensure fair comparison.

\subsection{Cross-Task Generalization to Tool Use and Coding}
\label{app:tool_coding_generalization}

One reviewer asked whether SAGE generalizes beyond mathematical reasoning. We therefore conducted additional experiments on coding and tool-use tasks with SAGE-RL. Specifically, we used TACO programming problems for training and LCBv6 programming problems for testing. We fine-tuned DS-1.5B with SAGE-GRPO and vanilla GRPO under the same inference settings.

\begin{table}[t]
  \centering
  \caption{Cross-task results on coding/tool-use style tasks. SAGE-GRPO improves accuracy and token efficiency while shortening responses relative to vanilla GRPO.}
  \label{tab:rebuttal_coding_tool}
  \begin{tabular}{lrrr}
    \toprule
    Model & Pass@1 (\%) & Len. & TE ($\times 10^{-3}$) \\
    \midrule
    DS-1.5B & 12.4 & 27659 & 0.448 \\
    +GRPO & 23.5 & 23847 & 0.985 \\
    +SAGE-GRPO & 27.7 & 12926 & 2.143 \\
    \bottomrule
  \end{tabular}
\end{table}

SAGE-GRPO improves Pass@1 by 4.2 points over GRPO and reduces average response length by 45.8\%, yielding a 117.6\% improvement in token efficiency. This suggests that the efficiency pattern learned through SAGE-RL transfers beyond the mathematical benchmarks used in the main experiments.

\subsection{Relation to DeepConf}
\label{app:deepconf_relation}

Reviewers also asked about the relation between SAGE and DeepConf. Both methods exploit confidence signals, but they operate at different levels. DeepConf primarily uses confidence to select among complete sampled outputs at inference time, whereas SAGE uses average cumulative log-probability $\Phi$ to guide step-wise exploration and then transfers this behavior into RL training through SAGE-RL. Thus, SAGE is not merely a filtering method over complete answers: it changes the rollout distribution during training so that the policy learns to generate shorter and more reliable reasoning paths under standard inference.

\subsection{Baseline Hyperparameter Tuning}
\label{app:baseline_tuning}

To address concerns about baseline tuning, we conducted hyperparameter ablations for SAGE-GRPO and additional baselines beyond GRPO, including AdaptThink and ThinkPrune-2k. We swept the learning rate over $\{5\times10^{-7}, 2\times10^{-6}\}$ and the KL coefficient over $\{5\times10^{-4}, 2\times10^{-3}\}$, training each method independently under each setting.

Across all four configurations, the relative ranking is stable: SAGE-GRPO consistently achieves the highest Pass@1 and token efficiency. AdaptThink and ThinkPrune obtain shorter responses in some cases, but this compression comes at an accuracy cost; both underperform vanilla GRPO in Pass@1. These results indicate that the improvements of SAGE-GRPO are not artifacts of a particular hyperparameter choice.

\subsection{Training Overhead}
\label{app:training_overhead}

We further report training memory and wall-clock cost to clarify the overhead introduced by SAGE sampling. The results are summarized in Table~\ref{tab:rebuttal_overhead}. With vLLM rollout, SAGE-GRPO has comparable peak GPU memory to GRPO and only moderate additional wall-clock time. Under HF inference, SAGE-GRPO uses moderately more memory but runs faster than GRPO, which is consistent with the reduction in generated tokens.

\begin{table}[t]
  \centering
  \caption{Training overhead comparison.}
  \label{tab:rebuttal_overhead}
  \begin{tabular}{llrr}
    \toprule
    Method & Rollout engine & Peak memory (MiB) & Time (h) \\
    \midrule
    GRPO & vLLM / verl & 70089 & 27.1 \\
    SAGE-GRPO & vLLM / verl & 70091 & 30.2 \\
    GRPO & HF & 36118 & 96.8 \\
    SAGE-GRPO & HF & 40020 & 93.2 \\
    ThinkPrune & vLLM / verl & 69991 & 29.5 \\
    LC-R1 & vLLM / verl & 70403 & 31.8 \\
    AdaptThink & vLLM / verl & 75613 & 33.8 \\
    \bottomrule
  \end{tabular}
\end{table}

Overall, SAGE-GRPO has competitive overhead compared with all baselines while preserving the main benefit of substantially improved token efficiency.
